# Supplementary material for: Orbital Graph Convolutional Neural Network for Material Property Prediction
Source: arXiv:2008.06415 source file (2020-08-14)
Supplement: Supplementary file 1 [file Supplementary_info_arxiv.pdf]

# Orbital Graph Convolutional Neural Network for Material Property Prediction

Mohammadreza Karamad[1,2,*], Rishikesh Magar[1,*], Yuting Shi[1], Samira Siahrostami[3], Ian D. Gates[2], and Amir Barati Farimani[1,†]

[1]Department of Mechanical Engineering, Chemical Engineering and Biomedical Engineering, Carnegie Mellon University, Pittsburgh, Pennsylvania 15213, United States

[2]Department of Chemical and Petroleum Engineering, University of Calgary, 2500 University Drive NW Calgary Alberta T2N 1N4 Canada

[3]Department of Chemistry, University of Calgary, 2500 University Drive NW, Calgary, Alberta T2N 1N4, Canada

[*]These authors contributed equally to this work.

[†]Corresponding author e-mail: barati@cmu.edu

# 1 SUPPLEMENTARY METHODS AND DISCUSSIONS

## 1.1 Model Architecture

The architecture of the Orbital Graph Convolutional Neural Network (OGCNN) model is shown in Figure S1.

We divide the architecture into 4 modules: (a) Input module, (b) Encoder-Decoder module, (c) Graph Convolution module, and (d) the Output module. The input module is depicted in detail in Figure S2. In the input module, for each atom in a crystal, three sets of features are considered: (1) $1 \times 92$ basic atomic features as in Table S1 (Ref [1]),(2) $32 \times 33$ Orbital Field Matrix (OFM) which encodes orbital-orbital interactions of center atom with neighbor atoms [2], and (3) $12 \times 92$ neighbor atom features which account for the basic atomic features of neighbor atoms. We only consider the first 12 nearest neighbor atoms. The list of 92 basic atomic features (elemental features) are provided in Table S1.

The Encoder-Decoder module learns important features among basic atomic features and OFM features. The encoder-decoder network which comprises of 1148 at the encoder input, 768 neurons in the hidden layer ($L1$) and 1536 neurons at decoder output ($L2$). In this module, the most significant features are selected. The output from the second layer is passed to graph convolution module. A softplus[3] activation is used between the layers of the encoder-decoder network. The performance improvement due to using an encoder-decoder network initially in our case can be seen from Figure S3(b) where 2 fully connected (FC) layers after the input clearly give an improved performance, helping us establish the importance of the addition of an encoder-decoder to the OGCNN model.

In Graph convolution module, for each atom in the crystal we concatenate the following vectors: 1) the $12 \times 1536$ resulted from the output of Encoder-Decoder module for the center

atom. We note that the center atom features are essentially $1 \times 1536$ but we repeat these features 12 times to construct $12 \times 1536$ arrays in order to ensure shape compatibility with neighbor features. 2)the $12 \times 1536$ resulted from the output of Encoder-Decoder module for neighbor atoms (1536 features for each neighbor atom), and 3) the $12 \times 41$ kernelized distance features corresponding to the 12 neighbor atoms of center atom (41 kernelized distance features for each neighbor atom). This also means, there are now $12 \times 3113$ features for each atom for each crystal in the batch. Then, we apply a fully connected layer which reduces the number of features from 3113 to 3072. Therefore, we end up with $12 \times 3072$ features for each atom in the batch. We then perform a convolutional operation on 3072 features by first splitting them into two equal sets, C anb N sets, followed by an element wise multiplication of C and N. The number of convolutions,R, for our network is 3. The number of convolutions, however, can be tuned and is a hyperparameter for the network. Finally, at the end of convolution module, a summation operation is performed over all the neighbors which results in a $1 \times 1536$ features for each atom. The output of the convolution module is passed to the output module.

The output module consists of a pooling layer and two fully connected layers. A pooling layer is used to map the properties from the atom level to the crystal level in the batch. This is done by using a mean pooling operation over the atoms in each crystal in a batch. After softplus activation [3], the output from the pooling layer is fed to the L3 layer with 128 neurons. We again apply a softplus activation to the output from L3 which is subsequently fed to the output layer with one neuron for property prediction.

## 1.2 Orbital Feature Matrix (OFM)

The OFM encodes the orbitals interactions, and captures the spatial and structural information by constructing Voronoi cells between center and neighbor atoms. The OFM corresponding to each atom is a $32 \times 33$ two-dimensional matrix. In order to combine these two sets of features, i.e. OFM and the basic atomic features, the OFM is flattened into a $1 \times 1056$ one-dimensional vector, and then is concatenated with $1 \times 92$ one-dimensional basic atomic features to form a $1 \times 1148$ one-dimensional atom features. It is worth mentioning that, one can convert the $32 \times 33$ two-dimensional OFM into a $1 \times 33$ one-dimensional matrix by summing or averaging over OFM columns. However, both summing and averaging operations resulted in lower performance, presumably due to loss of information.

## 1.3 Choice of Optimizer

During training the OGCNN model, mean square loss (MSE) as a loss function and stochastic gradient descent (SGD) as an optimizer have been used. We also considered using Adam as an optimizer, but SGD showed a better performance. For example, by using the Adam optimizer for Lanthanides dataset we obtained a MAE value of 0.095 for test set, while using the same hyperparameters with the SGD, we obtained a MAE value of 0.072 for the test set.

## 1.4 Hyperparameters Optimization

We used Perovskites dataset and Lanthanides datasets in order to optimize hyperparameters in the OGCNN model. First, as explained above in the Model Architecture section, in order to extract important features among center and neighbor atoms feature, we used an encoder-decoder style architecture. The encoder input has 1148 flattened basic atomic features and OFM features.The hidden layer (L1) has 768 neurons and decoder output has 1536 neurons,

respectively. The intuition behind the number of neurons came from our initial findings when we used only one fully connected layer during training. We tuned the number of neurons in the layer, by examining different sizes of hidden layers varying from 100 to 1100 with steps of 200 (Figure S3(a)) We found that by increasing the number of neurons the MAE value is decreased. Moreover, we found that 800 neurons resulted in both high performance and faster computation compared to the case with more hidden neurons (Figure S3b). Therefore, the number of neurons for our first fully connected layer was set to be close to 800. Subsequently, we increased the number of layers in order to have an encoder-decoder like structure that can select more important features. The number of neurons for the second fully connected layer was set to double the number of neurons in the first fully connected layer which is a common convention in neural network architectures. We also tried different number of neurons in the second layer, but the best results (lowest MAE values) were achieved for 1536 neurons. We increased the neuron size in the second layer to 1200,1400,1600,1800,2000, and we did not observe significant reduction in the MAE values by increasing the number of neurons in the second hidden layer. The results of our experiments with the number of neurons in the second hidden layer are shown in Figure S4(b). Moreover, since we are interested only in the regression tasks, MSE loss was chosen when training the model. The training curve for the OGCNN model for Perovskites dataset is provided in Figure S4(a). It must be noted that the model parameters at the epoch where lowest validation MAE is observed are chosen to evaluate on the test set. In addition to tuning the OGCNN for hyperparameters like learning rate $\alpha$, number of hidden layers, number of hidden units, momentum, batch size and weight decay, we evaluated the performance of the OGCNN model when: 1) different number of neighbors is selected , 2) different distance dependent weight functions, $\zeta(r_{cn})$, and 3) different sizes of fully connected neurons with different number of layers used during training process. Figure S5a shows the performance of the OGCNN model in training Perovskites dataset when different number of neighbors is selected. As can be seen, the MAE values marginally change by increasing the number of neighbors beyond 12. Figure S5b shows the performance of the OGCNN model in training Lanthanides dataset using different $\zeta(r_{cn})$ functions. We observed that using $\frac{1}{r_{cn}^4}$ as distance function resulted in the highest performance among all examined distance functions. In addition, we compared the performance of our model without applying any fully connected layer (Figure S3(b)). It is seen that the accuracy of the OGCNN model is higher than that of for CGCNN model even without applying any fully connected layer. Figure S3(b) helps us essentially validate that the performance of OGCNN improves with the encoder- decoder layer as it can be seen from Fig.S3(b) that two FC layers after flattened features has the lowest MAE.

## 1.5 Cross Validation

The cross validation is used in this work to ensure robustness in predictions of the machine learning model. The conventional idea of cross validation is to check the effectiveness of model against different test sets and also attenuate overfitting in some cases. In cross validation, a subset of the data is held as the test set and the rest of the dataset is the training data for the model. We do cross validation to remove any bias that we may have when evaluating the model. When we evaluate the performance of the model against different test sets, we can gauge the performance of the model better which leads to a more robust and accurate estimate of the performance.

### 1.6 Learning Curves

In order to make sure that the OGCNN model is not overfitting, we have plotted the training and validation loss when training different datasets in Figure S7. The plots are indicative that the model is not necessarily overfitting but learning material representation from training set and is able to generalize well on validation and test sets.

## 2 Datasets

To train the OGCNN model, we used the following Density Functional Theory (DFT)-calculated databases.
1- **MP-formation energy** [4]: This dataset consists of formation energies of 26741 crystalline systems from the Materials Project database.

2- **Lanthanides** [2]: This dataset consists of formation energies of 4191 transition metal binary alloys (TT), bimetal alloys of lanthanide metal and transition metal (LATX), and the LATX and TTX which are the LAT and TT alloys that include X element. The transition metals are from the set of Sc, Ti,V,Cr, Mn, Fe, Co,Ni, Cu,Zn, Y, Zr,Nb, Mo, Tc, Ru, Rh, Pd, Ag, Cd, Hf, Ta,W, Re, Os, Ir, Pt, Au, the lanthanides are from La, Ce, Pr, Nd, Pm, Sm, Eu, Gd,Tb, Dy, Ho, Er, Tm, Yb, Lu, and the X elements are from B, C, N, O.

3- **Perovskites** [5]: This dataset consist of formation energies of 18928 cubic perovskites with general formula ABX3, where A and B elements are from any nonradioactive metals, and X can be one or several elements from O, N, S, and F. The cubic Perovskites in this dataset cover 52 metals.

4- **MP-Fermi energy** [4]: This dataset consists of Fermi energies of 26447 crystalline systems from the Materials Project database.

5- **MP-band gap** [4]: This dataset consists of band gap energies of 27111 crystalline systems from the Materials Project database.

## 3 2D histograms for predicted properties against DFT-calculated values

Figure S6 shows the comparison between the DFT-calculated values and predicted properties using OGCNN for (a) Perovskites, (b) MP-Fermi energy, (c) MP-formation energy and (d) MP-band gap datasets.

## 4 Smooth Overlap of Atomic Positions (SOAP) and Many-body Tensor Representation (MBTR) descriptors optimization

We benchmarked our results against two previously developed state-of-the-art descriptors for encoding atomic structures including the Many-Body Tensor Representation (MBTR) that encodes the periodic crystalline structures as a whole by expanding them in a distribution of different structural motifs that are based on chemical elements, and 2) the Smooth Overlap of Atomic Positions (SOAP) that encodes the local chemical environments of a center atom as smoothed Gaussian densities of neighboring atoms. The SOAP and MBTR hyperparameters

were optimized for each property following Ref.[6] to assure maximum accuracy when training our datasets [6, 7, 8].

### 4.1 SOAP:

To optimize SOAP hyperparameters, following Ref. [6], we fixed the number of radial basis functions and the maximum degree of spherical harmonics at $n_{max} = 8$ and $l_{max} = 8$, respectively. To find optimal values for both $\sigma$, the width of the gaussian smoothing, and $r_{cut}$, the radial cut off value, we performed a grid search for different combinations of $\sigma$ and $r_{cut}$. Moreover, we used "gto" as the Spherical Gaussian type orbitals as the radial basis functions for SOAP ($SOAP_{gto}$). We tested each set of SOAP hyperparameters in the grid using 'rbf' Kernel Ridge Regression (KRR). Once we find the optimal values for SOAP hyperparameters, we use KRR to train each dataset. We performed two different grids search to find optimal KRR hyperparameters: 1) a two-dimensional logarithmic grid using spacing factor of 10 and 2 for the kernel width $\gamma$ and the regularization parameter $\alpha$,respectively, and 2) a two-dimensional grid using a logarithmic grid with spacing factor of 2 for the kernel width $\gamma$ and a linear grid for regularization parameter $\alpha$. For each set of hyperparameteres in the grids, we performed a 5-fold cross-validation by splitting each dataset to 80% and 20% for train and test sets, respectively. Table S2 shows the optimal values for SOAP hyperparameters for each dataset along with the lowest MAE values obtained when training our datasets using SOAP.

### 4.2 MBTR:

Following Himanen et al. [6], for each dataset, when using MBTR descriptor we optimized: $\sigma_k$ that is the standard deviation of the gaussian distribution, and $s_k$ that is the factor used in exponential weighting. To find optimal hyperparameters for MBTR, we examined different values for both $\sigma_k$ and $s_k$ for each k-term separately. We then used these optimal values to train our datasets using MBTR descriptor and 'rbf' KRR. We performed two different grids search to find optimal KRR hyperparameters: 1) a two-dimensional logarithmic grid using spacing factor of 10 and 2 for the kernel width $\gamma$ and the regularization parameter $\alpha$,respectively, and 2) a two-dimensional grid using a logarithmic grid with spacing factor of 2 for the kernel width $\gamma$ and a linear grid for regularization parameter $\alpha$. For each set of hyperparameters in the grids, we performed a 5-fold cross-validation by splitting each dataset to 80% and 20% for train and test sets, respectively[9]. Table S3 shows the optimal values for $\sigma_k$ and $s_k$ for each k-term for different datasets along with the lowest MAE values obtained when training our datasets using MBTR descriptor.

We would like to emphasize that SOAP performed better than CGCNN for all predicted properties. On the contrary, MBTR performance was lower than CGCNN for all predicted properties with the exception of the formation energy of perovskites where the MBTR showed higher performance than CGCNN. We note that the performance of MBTR and SOAP descriptors depend on several hyperparameters that are dataset-specific, and these hyperparameters need to be optimized before used for training. On the other hand, the OGCNN does not require dataset-specific optimization making it faster when used to predict material properties.

## 5 SUPPLEMENTARY FIGURES

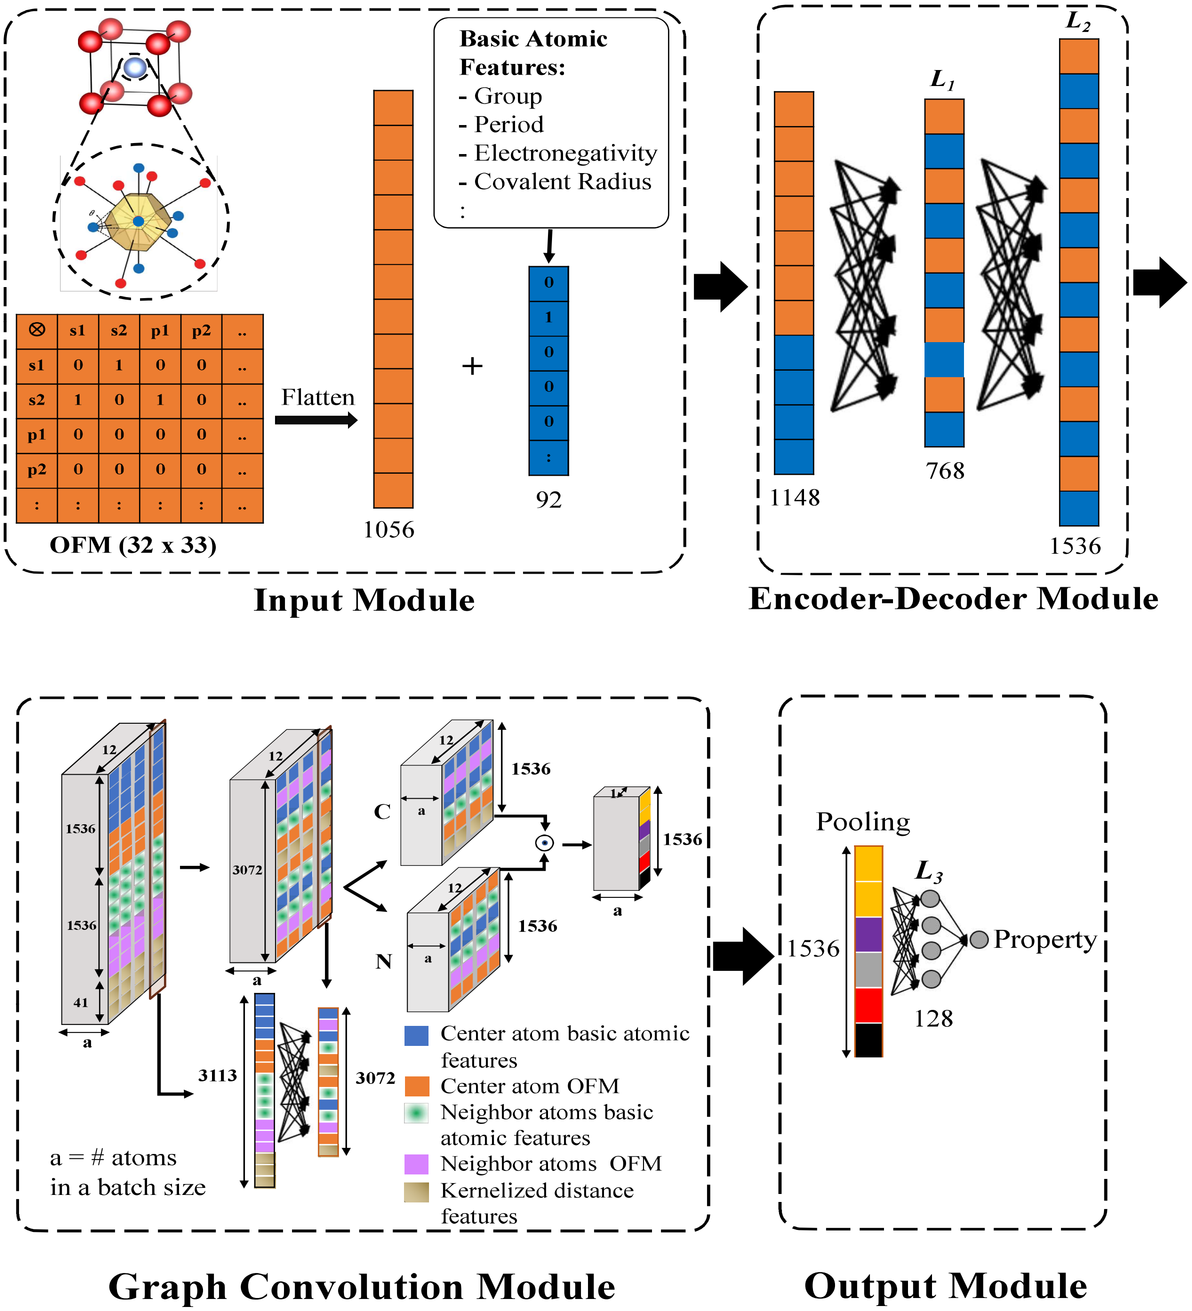


**Figure S 1.** Structure of the OGCNN framework as applied in this Letter.

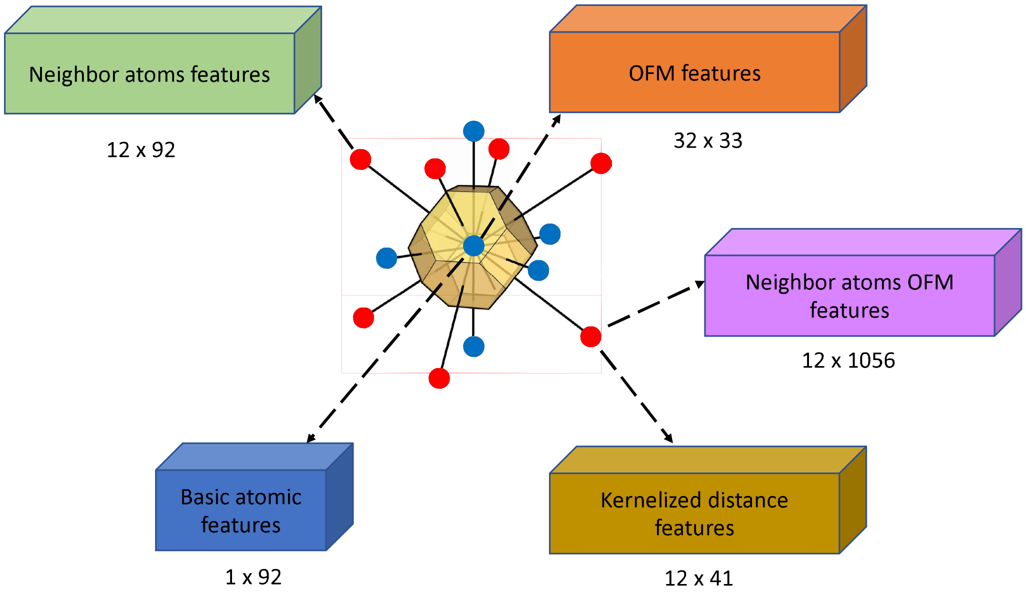


**Figure S 2.** List of different features used in the OGCNN model.

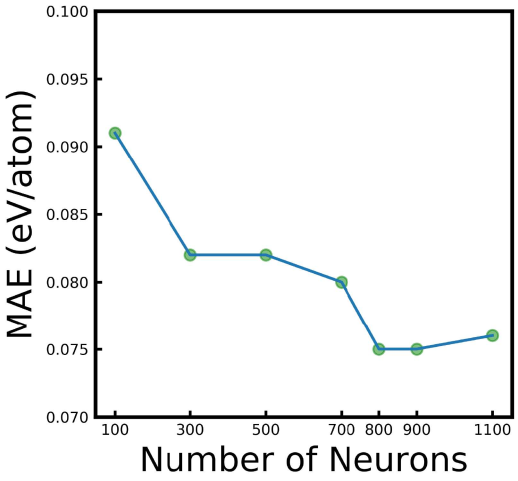


**(a)**

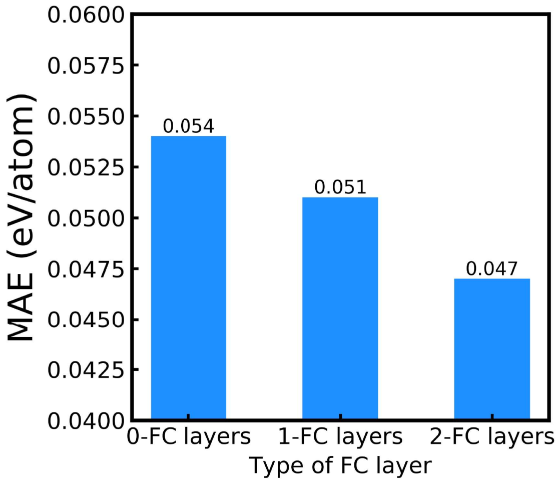


**(b)**

**Figure S 3.** (a) The MAE values when applying one fully connected (FC) layer to learn important features from the flattened features is plotted against the number of neurons in the layer. The training was performed for the Lanthanides dataset. (b) The MAE trend showing how the accuracy of prediction changing with the number of fully connected layers after the flattened features for the Pervoskites dataset.

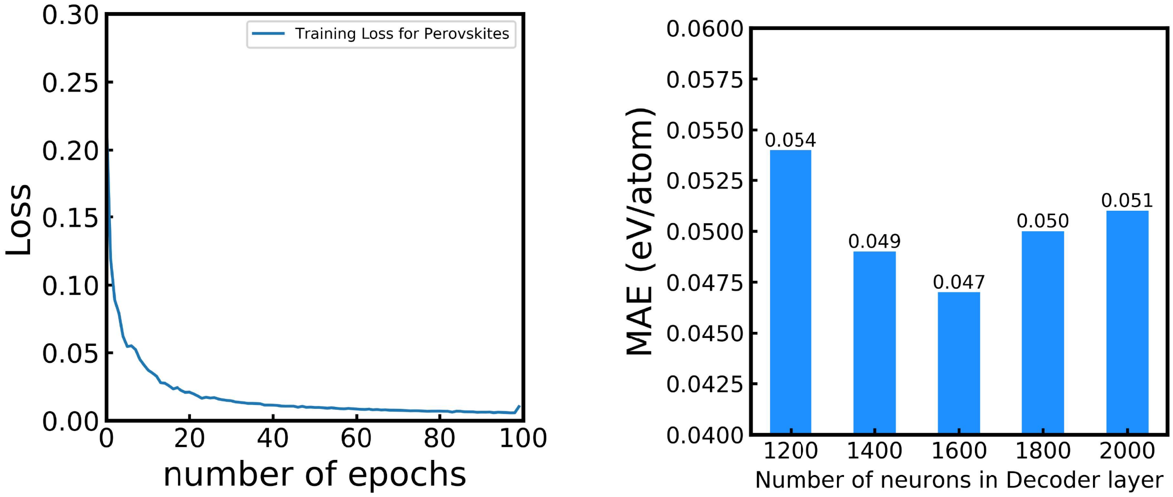


**(a)** **(b)**

**Figure S 4.** (a) The training loss vs epoch plot for the Perovskites dataset .(b) The MAE values are plotted against the number of neurons in the decoder layer. The number of neurons are varied from 1200 to 2000 with a step size of 200.

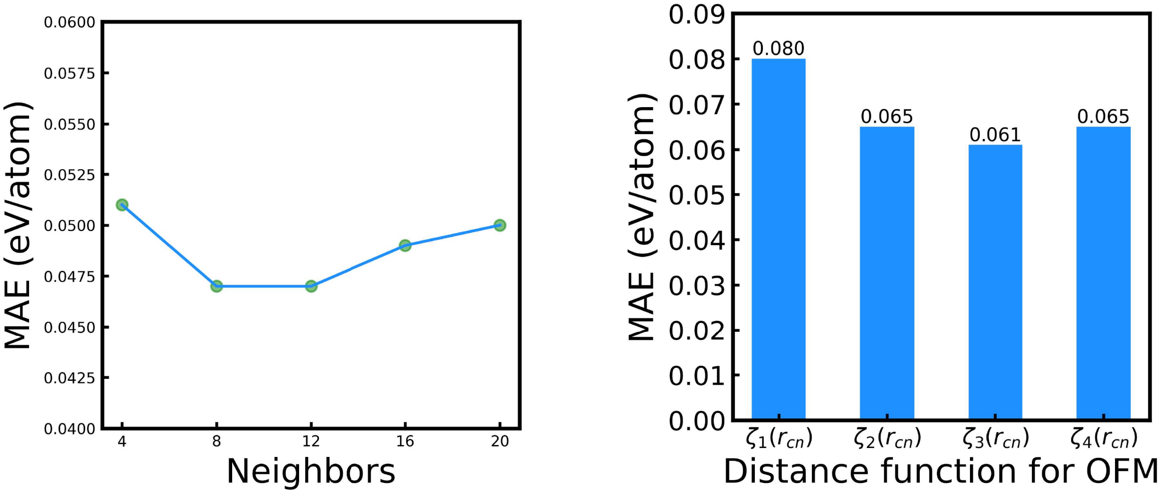


**(a)** **(b)**

**Figure S 5.** (a) The average of the MAE values against the number of nearest neighbors for training Perovskites datasets using OGCNN. (b) MAE values when training Perovskites dataset with OGCNN model using different distance functions. The $\zeta_1(r_{cn})$, $\zeta_2(r_{cn})$, $\zeta_3(r_{cn})$, and $\zeta_4(r_{cn})$ in the legend correspond to $\frac{1}{r_{cn}}$, $\frac{1}{r_{cn}^2}$, $\frac{1}{r_{cn}^4}$, and $\frac{1}{r_{cn}^6} - \frac{1}{r_{cn}^{12}}$ distance functions, respectively.

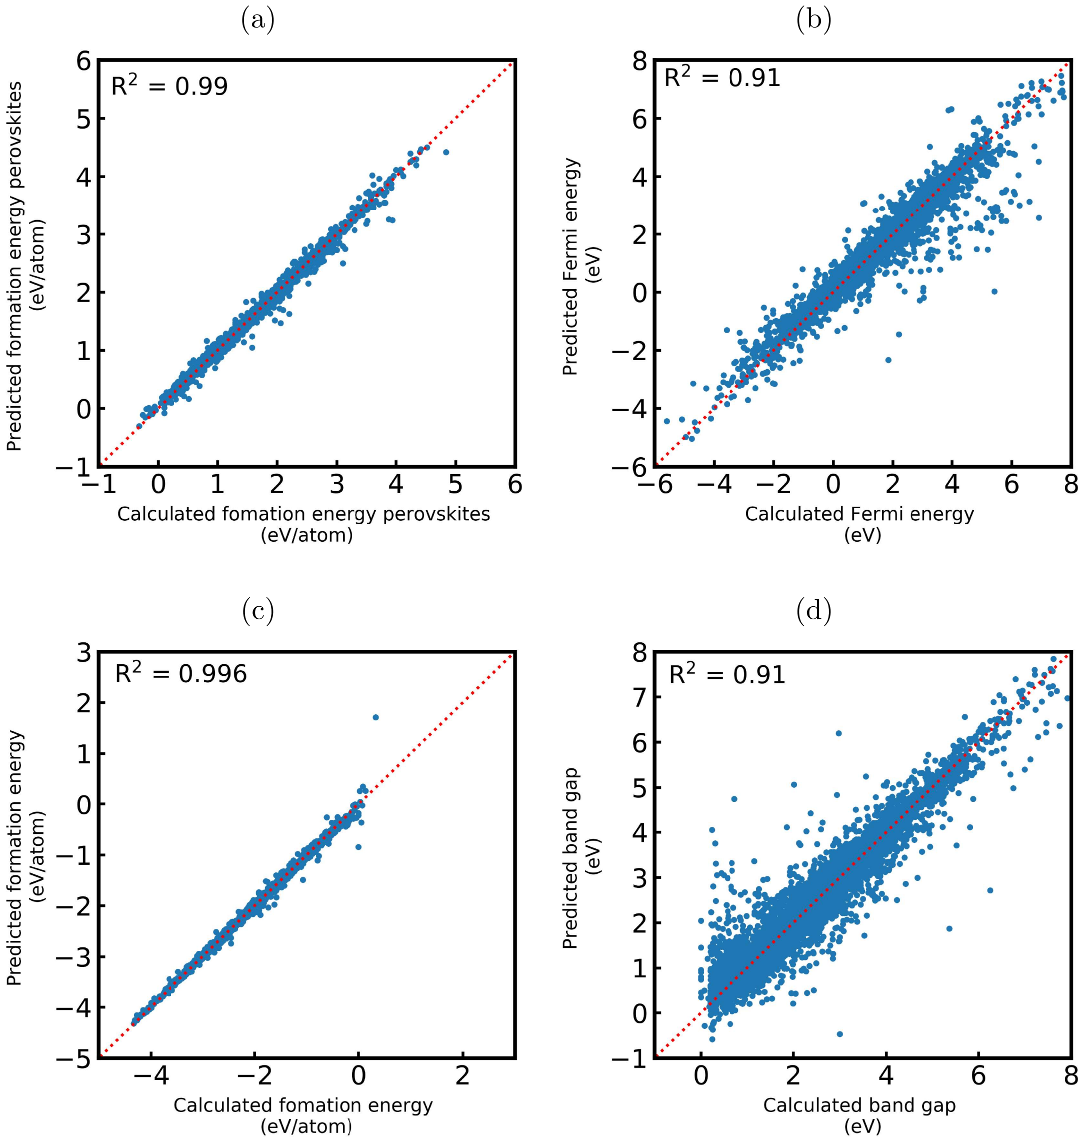


**Figure S 6.** Comparison between the ground truth values (DFT-calculated) and predicted values using OGCNN model for test sets of: (a) formation energy of Perovskites, (b) MP-Fermi energy, (c) MP-formation energy, and (d) MP-band gap.

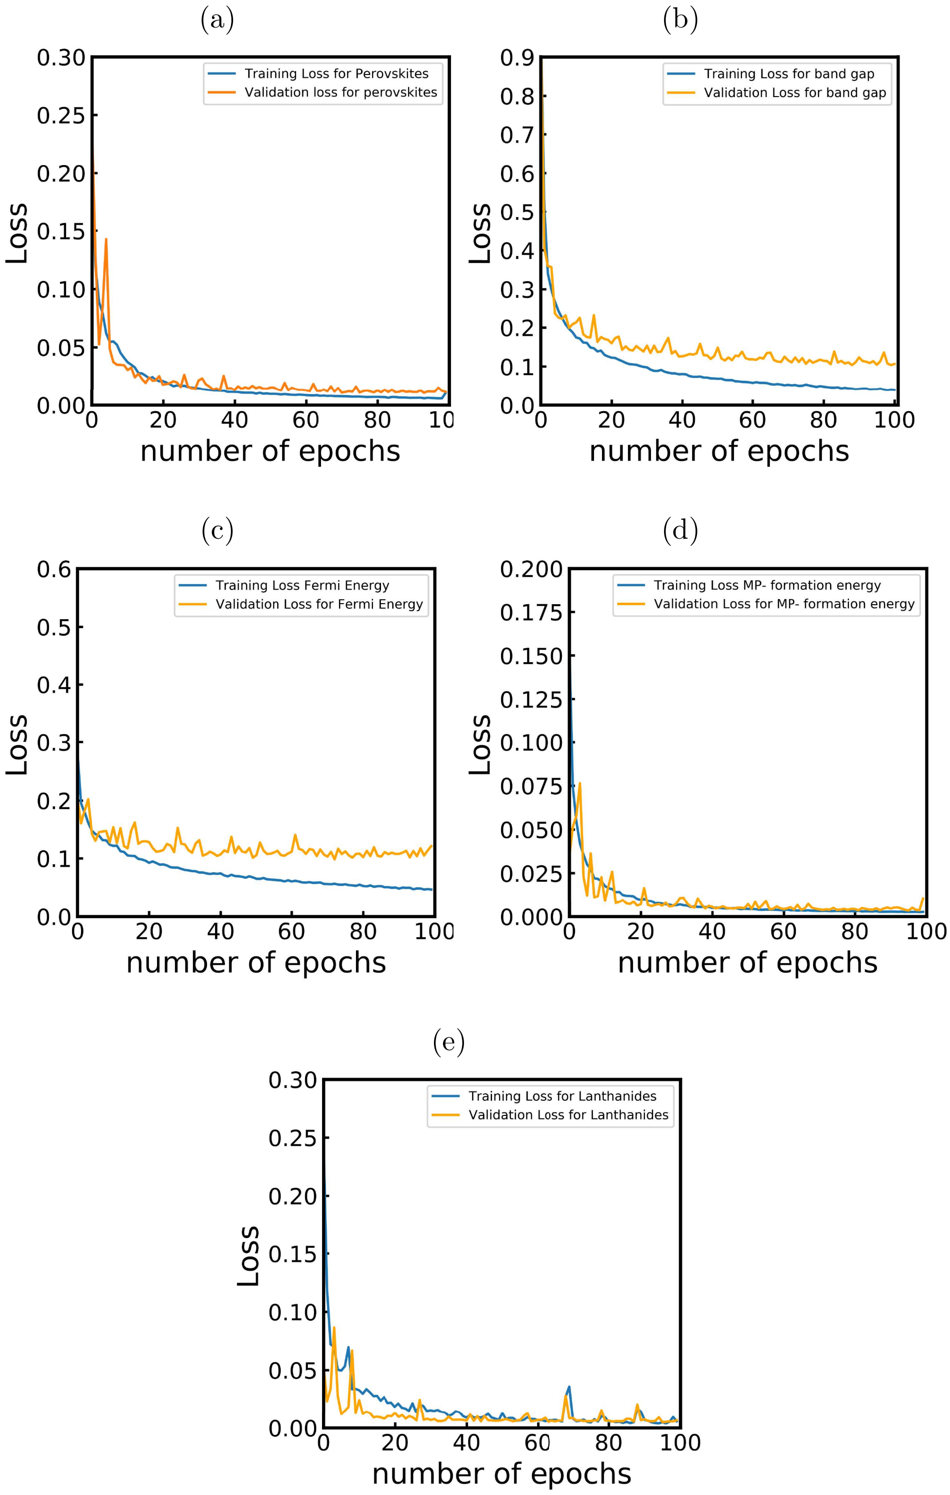


**Figure S 7.** Training and validation loss for (a) Perovskites,(b) band gap, (c) Fermi energy, (d) MP- formation energy,(e) Lanthanides .

# 6 SUPPLEMENTARY TABLES

Table S1: Basic atomic features used in OGCNN model [1]

| Property | Unit | Range | (#) of categories |
|---|---|---|---|
| Group Number | - | 1,2,3.....,18 | 18 |
| Period Number | - | 1,2,3,....,9[a] | 9 |
| Electronegativity | - | 0.5-40 | 10 |
| Covalent Radius | pm | 25-250 | 10 |
| Valence Electron | - | 1,2,3....,12 | 12 |
| First Ionization energy | eV | 1.3-3.3 | 10 |
| Electron Affinity | eV | -3-3.7 | 10 |
| Block | - | s,p,d,f | 4 |
| Atomic Volume[b] | $cm^3/mol$ | 1.5-4.3 | 10 |

a: The lanthanide and actinide elements are considered as period 8 and 9 respectively
b: Log scale is used for these properties

Table S2: The optimization grid for the SOAP hyperparameters. The Spherical gaussian type orbitals were used as radial basis functions, and the average output for all selected positions were calculated. $l_{max}$, $n_{max}$, $r_{cut}$ and $\sigma$ are the number of radial basis functions, the maximum degree of spherical harmonics, the radial cut off, and the width of the gaussian smoothing values, respectively. The optimal values are marked in bold. The lowest MAE values using SOAP descriptors and after optimizing the KRR hyperparameters with 5-fold cross-validation for each dataset are also provided.

| Dataset | SOAP hyperparameters | | | | MAE |
|---|---|---|---|---|---|
| | $l_{max}$ | $n_{max}$ | $r_{cut}(\mathring{A})$ | $\sigma(\mathring{A})$ | |
| Lanthanides -formation energy | 8 | 8 | [**4**,6,8,10] | [0.8, **0.4**, 0.2, 0.1, 0.05] | 0.09 ($eV/atom$) |
| Perovskites -formation energy | 8 | 8 | [4,**6**,8,10] | [0.8, 0.4, **0.2**, 0.1, 0.05] | 0.11 ($eV/atom$) |
| MP-formation energy | 8 | 8 | [4,**6**,8,10] | [0.8, 0.4, **0.2**, 0.1, 0.05] | 0.05 ($eV/atom$) |
| MP-band gap | 8 | 8 | [4,6,8,**10**] | [0.8, 0.4, **0.2**, 0.1, 0.05] | 0.44($eV$) |
| MP-Fermi energy | 8 | 8 | [4,**6**,8,10] | [0.8, 0.4, **0.2**, 0.1, 0.05] | 0.38 ($eV$) |

Table S3: The optimization grid for MBTR hyperparameters. $\sigma_k$ is the standard deviation of the gaussian distribution and $s_k$ is the factor used in exponential weighting. The optimal values are marked in bold. The lowest MAE values using MBTR descriptors and after optimizing the KRR hyperparameters with 5-fold cross-validation for each dataset are also provides.

| Dataset | MBTR hyperparameters | | | MAE |
|---|---|---|---|---|
| | k-term | $\sigma_k$ | $s_k$ | |
| Lanthanides | | | | |
| -energy | $k_1$ | [0.4, 0.5, 0.6, **0.7**, 0.8, 0.9] | - | 0.28 $eV/atom$ |
| | $k_2$ | [0.005, 0.01, **0.02**, 0.04, 0.08] | [0.5, 0.6, 0.7, **0.8**] | |
| | $k_3$ | [**0.00025**, 0.0005, 0.001, 0.002, 0.004] | [0.25, 0.3, 0.35, **0.4**] | |
| Perovskites | | | | |
| -energy | $k_1$ | [0.4, 0.5, 0.6, **0.7**, 0.8, 0.9] | - | 0.091 $eV/atom$ |
| | $k_2$ | [0.005, 0.01, **0.02**, 0.04, 0.08] | [0.5, 0.6, 0.7, **0.8**] | |
| | $k_3$ | [**0.00025**, 0.0005, 0.001, 0.002, 0.004] | [0.25, 0.3, 0.35, **0.4**] | |
| MP | | | | |
| -energy | $k_1$ | [0.4, 0.5, 0.6, **0.7**, 0.8, 0.9] | - | 0.20 $eV/atom$ |
| | $k_2$ | [0.005, 0.01, **0.02**, 0.04, 0.08] | [0.5, 0.6, 0.7, **0.8**] | |
| | $k_3$ | [**0.00025**, 0.0005, 0.001, 0.002, 0.004] | [0.25, 0.3, 0.35, **0.4**] | |
| MP | | | | |
| -band gap | $k_1$ | [**0.4**, 0.5, 0.6, 0.7, 0.8, 0.9] | - | 0.69 $eV$ |
| | $k_2$ | [0.005, 0.01, 0.02, 0.04, **0.08**] | [0.5, 0.6, 0.7, **0.8**] | |
| | $k_3$ | [0.00025, 0.0005, **0.001**, 0.002, 0.004] | [0.25, 0.3, 0.35, **0.4**] | |
| MP | | | | |
| -Fermi | $k_1$ | [0.4, 0.5, 0.6, **0.7**, 0.8, 0.9] | - | 0.82 $eV$ |
| | $k_2$ | [**0.005**, 0.01, 0.02, 0.04,0.08] | [**0.5**, 0.6, 0.7, 0.8] | |
| | $k_3$ | [0.00025, 0.0005, 0.001, **0.002**, 0.004] | [0.25, 0.3, **0.35**, 0.4] | |

Table S4: Summary of the prediction performance of five different properties on test sets using the OGCNN and CGCNN. In addition, the MAE values for DFT calculations are provided. MP stands for Materials Project. We would like to emphasize that MP-formation energy, MP-Fermi energy datasets are slightly different from the ones in Ref.[1]. Therefore, we used CGCNN from the github repository given by the authors in the paper [1] to train these datasets.

| Dataset/Property | dataset size | Unit | epochs | MAE (OGCNN) | MAE (CGCNN) | MAE (DFT) |
|---|---|---|---|---|---|---|
| Lanthanides-formation energy | 4191 | eV/atom | 100 | 0.06 | 0.13 | 0.081-0.136 [10] |
| Perovskites-formation energy | 18928 | eV/atom | 100 | 0.05 | 0.09 | N/A |
| MP-formation energy | 26741 | eV/atom | 100 | 0.03 | 0.05 | 0.081-0.136 [10] |
| MP-band gap | 27111 | eV | 100 | 0.32 | 0.43 | 0.6 [11] |
| MP-Fermi energy | 26447 | eV | 100 | 0.038 | 0.43 | N/A |

# References


[1] T. Xie and J. C. Grossman, "Crystal graph convolutional neural networks for an accurate and interpretable prediction of material properties," *Phys. Rev. Lett.*, vol. 120, p. 145301, Apr 2018.

[2] T. L. Pham, H. Kino, K. Terakura, T. Miyake, K. Tsuda, I. Takigawa, and H. C. Dam, "Machine learning reveals orbital interaction in materials," *Science and Technology of Advanced Materials*, vol. 18, no. 1, pp. 756–765, 2017.

[3] A. B. Xavier Glorot and Y. Bengio, "Deep sparse rectifier neural networks," in *Proceedings of the 14thInternational Conference on Artificial Intelligence and Statistics (AISTATS).*

[4] A. Jain, S. P. Ong, G. Hautier, W. Chen, W. D. Richards, S. Dacek, S. Cholia, D. Gunter, D. Skinner, G. Ceder, and K. A. Persson, "Commentary: The materials project: A materials genome approach to accelerating materials innovation," *APL Materials*, vol. 1, no. 1, p. 011002, 2013.

[5] I. E. Castelli, T. Olsen, S. Datta, D. D. Landis, S. Dahl, K. S. Thygesen, and K. W. Jacobsen, "Computational screening of perovskite metal oxides for optimal solar light capture," *Energy Environ. Sci.*, vol. 5, pp. 5814–5819, 2012.

[6] L. Himanen, M. O. Jäger, E. V. Morooka, F. F. Canova], Y. S. Ranawat, D. Z. Gao, P. Rinke, and A. S. Foster, "Dscribe: Library of descriptors for machine learning in materials science," *Computer Physics Communications*, vol. 247, p. 106949, 2020.

[7] H. Huo and M. Rupp, "Unified representation of molecules and crystals for machine learning," 2017.

[8] A. P. Bartók, R. Kondor, and G. Csányi *Phys. Rev. B*, vol. 87, p. 184115, May 2013.

[9] P. Refaeilzadeh, L. Tang, and H. Liu, *Cross-Validation*, pp. 532–538. Boston, MA: Springer US, 2009.

[10] S. Kirklin, J. E. Saal, B. Meredig, A. Thompson, J. W. Doak, M. Aykol, S. Rühl, and C. Wolverton, "The open quantum materials database (oqmd): assessing the accuracy of dft formation energies," *npj Computational Materials*, vol. 1, p. 15010, Dec 2015.

[11] A. Jain, G. Hautier, C. J. Moore, S. P. Ong], C. C. Fischer, T. Mueller, K. A. Persson, and G. Ceder, "A high-throughput infrastructure for density functional theory calculations," *Computational Materials Science*, vol. 50, no. 8, pp. 2295 – 2310, 2011.
